# Supplementary material for: Combining Localized Orbital Scaling Correction and Bethe-Salpeter Equation for Accurate Excitation Energies
Source: arXiv:2207.00508 ancillary file (2022-07-01)
Supplement: Supplementary file 1 [file si.pdf]

# Supporting Information: Combining Localized Orbital Scaling Correction and Bethe-Salpeter Equation for Accurate Excitation Energies

Jiachen Li, Ye Jin, Neil Qiang Su, and Weitao Yang*

*Department of Chemistry, Duke University, Durham, NC 27708, USA*

E-mail: weitao.yang@duke.edu

## 1 Scaling Analysis of LOSC

The implementation of LOSC is very efficient. We begin with the scaling analysis of computing the local occupation matrix $\lambda$. We can express $\lambda$ by the unitary transformation matrix $U$

$$\lambda_{pq} = \sum_r \langle \varphi_p | \psi_r \rangle \langle \psi_r | \varphi_q \rangle = \sum_r U_{qr} U_{rp}. \tag{1}$$

Thus, the scaling of computing $\lambda$ is $O(N^3)$.

In the calculation of the curvature matrix $\kappa$, two-electron integrals in the first part are evaluated with resolution of identity (RI)

$$\iint \mathrm{d}r\, \mathrm{d}r' \frac{\rho_p(r)\rho_q(r')}{|r - r'|} = \langle \varphi_p \varphi_q | \varphi_p \varphi_q \rangle \tag{2a}$$

$$= \sum_P R_{P,pp} R_{P,qq}, \tag{2b}$$

where $R_{P,pq} = \sum_Q (P|Q)^{-\frac{1}{2}}(Q|rs)$ is constructed in the RI approximation and $\{\psi_Q\}$ is a set of auxiliary basis sets. The scaling for computing this part in the curvature matrix $\kappa$ is $O(N^3)$ and for forming three-center integrals in RI is $O(N^4)$. The second part in the curvature matrix can be efficiently done by the numerical integration of a scaling $O(N_{\mathrm{grid}}N)$, where $N_{\mathrm{grid}}$ is number of grid points in real space. With the $\lambda$ and $\kappa$ matrices, it is clear that the formulation of the LOSC effective Hamiltonian $\Delta h^{\mathrm{LOSC}}$ is of a $O(N^2)$ scaling.

For the restrained Boys localization, the computational cost of a single iteration to evaluate the target function $F$ is $O(N_{\mathrm{grid}}N)$ for the physical space integral and $O(N^2)$ for the energy space integral.

Therefore, the overall of the LOSC method itself scales $O(N^3)$ with respect to the size of the system (if three-center integrals in RI are not constructed). The scaling is $O(N^4)$ if we need to construct RI integrals.

## 2 Results of Truhlar-Gagliardi Test Set

**Table S1:** Excitation energies of molecules in the Truhlar-Gagliardi test set[S1] obtained from BSE/post-LOSC and BSE-TDA/post-LOSC based on different starting points. The aug-cc-pVTZ basis set was used except for naphthalene, pNA and DMABN that were calculated with the aug-cc-pVDZ basis set. B-TCNE was not included because of computational cost. All values in eV.

| | | | BSE/post-LOSC | | | | BSE-TDA/post-LOSC | | | |
|---|---|---|---|---|---|---|---|---|---|---|
| | state | ref | BLYP | PBE | B3LYP | PBE0 | BLYP | PBE | B3LYP | PBE0 |
| acetaldehyde | $^1A''$ | 4.31 | 3.53 | 3.42 | 4.01 | 4.06 | 3.58 | 3.47 | 4.05 | 4.11 |
| acetone | $^1A_2$ | 4.47 | 3.93 | 3.86 | 4.31 | 4.37 | 3.97 | 3.91 | 4.35 | 4.41 |
| formaldehyde | $^1A_2$ | 3.98 | 2.65 | 2.53 | 3.19 | 3.27 | 2.71 | 2.60 | 3.25 | 3.33 |
| pyrazine | $^1B_{3u}$ | 4.15 | 3.70 | 3.72 | 4.27 | 4.44 | 3.93 | 3.95 | 4.49 | 4.58 |
| pyridazine | $^1B_1$ | 3.83 | 2.43 | 2.32 | 3.22 | 3.35 | 2.57 | 2.46 | 3.34 | 3.45 |
| pyridine | $^1B_1$ | 4.95 | 4.10 | 4.12 | 4.53 | 4.69 | 4.22 | 4.24 | 4.63 | 4.79 |
| pyrimidine | $^1B_1$ | 4.44 | 4.13 | 3.99 | 4.66 | 4.68 | 4.19 | 4.04 | 4.71 | 4.73 |
| s-tetrazine | $^1B_{3u}$ | 2.47 | 0.87 | 0.66 | 1.66 | 1.69 | 1.06 | 0.88 | 1.79 | 1.82 |

**Table S1:** Continued

| | state | ref | BSE/post-LOSC | | | | BSE-TDA/post-LOSC | | | |
|---|---|---|---|---|---|---|---|---|---|---|
| | | | BLYP | PBE | B3LYP | PBE0 | BLYP | PBE | B3LYP | PBE0 |
| ethylene | $^1B_{3u}$ | 7.93 | 5.86 | 5.77 | 6.67 | 6.80 | 5.91 | 5.82 | 6.71 | 6.84 |
| butadiene | $^1B_u$ | 6.22 | 5.40 | 5.35 | 5.40 | 5.47 | 5.96 | 5.81 | 5.99 | 6.06 |
| benzene | $^1B_{2u}$ | 5.06 | 3.83 | 3.85 | 4.42 | 4.60 | 3.88 | 3.90 | 4.47 | 4.64 |
| | $^3B_{1u}$ | 4.16 | 1.93 | 1.96 | 2.66 | 2.86 | 2.56 | 2.58 | 3.16 | 3.33 |
| naphthalene | $^1B_{3u}$ | 4.00 | 3.97 | 4.09 | 4.27 | 4.37 | 4.15 | 4.30 | 4.35 | 4.43 |
| | $^3B_{2u}$ | 3.11 | 2.07 | 2.22 | 2.43 | 2.56 | 2.45 | 2.57 | 2.76 | 2.87 |
| furan | $^1B_2$ | 6.37 | 5.28 | 5.28 | 5.55 | 5.63 | 5.58 | 5.76 | 5.75 | 5.90 |
| | $^3B_2$ | 4.20 | 2.60 | 2.62 | 2.93 | 3.02 | 2.97 | 2.99 | 3.25 | 3.33 |
| hexatriene | $^1B_u$ | 5.37 | 4.73 | 4.74 | 4.82 | 4.83 | 5.26 | 5.27 | 5.32 | 5.33 |
| | $^3B_u$ | 2.73 | 1.66 | 1.66 | 1.92 | 1.95 | 2.20 | 2.19 | 2.37 | 2.39 |
| water | Singlet | 7.62 | 6.95 | 7.12 | 7.48 | 7.74 | 7.00 | 7.17 | 7.53 | 7.78 |
| | Triplet | 7.25 | 6.08 | 6.24 | 6.69 | 6.98 | 6.13 | 6.29 | 6.73 | 7.02 |
| pNA | $^1A_1$ | 4.39 | 3.65 | 3.75 | 4.11 | 4.23 | 3.80 | 3.89 | 4.23 | 4.35 |
| DMABN | $^1A_1$ | 4.86 | 4.06 | 3.99 | 4.33 | 4.39 | 4.15 | 4.08 | 4.41 | 4.49 |

**Table S2:** Excitation energies of molecules in the Truhlar-Gagliardi test set[S1] obtained from BSE/SCF-LOSC and BSE-TDA/SCF-LOSC based on different starting points. The aug-cc-pVTZ basis set was used except for naphthalene, pNA and DMABN that were calculated with the aug-cc-pVDZ basis set. B-TCNE was not included because of computational cost. All values in eV. Some results are missing because of the convergence issue in SCF-LOSC.

| | state | ref | BSE/SCF-LOSC | | | | BSE-TDA/SCF-LOSC | | | |
|---|---|---|---|---|---|---|---|---|---|---|
| | | | BLYP | PBE | B3LYP | PBE0 | BLYP | PBE | B3LYP | PBE0 |
| acetaldehyde | $^1A''$ | 4.31 | 3.52 | 3.40 | 4.02 | 5.83 | 3.57 | 3.45 | 4.06 | 5.87 |
| acetone | $^1A_2$ | 4.47 | | | 4.49 | | | | 4.53 | |
| formaldehyde | $^1A_2$ | 3.98 | 2.67 | 2.55 | 3.23 | 5.15 | 2.73 | 2.61 | 3.29 | 5.20 |
| pyrazine | $^1B_{3u}$ | 4.15 | | | | | | | | |
| pyridazine | $^1B_1$ | 3.83 | | 2.30 | 3.22 | 4.72 | | 2.45 | 3.33 | 4.81 |
| pyridine | $^1B_1$ | 4.95 | 4.09 | | | | | | | |
| pyrimidine | $^1B_1$ | 4.44 | 4.12 | | | 6.13 | 4.17 | | | |
| s-tetrazine | $^1B_{3u}$ | 2.47 | | | | | | | | |
| ethylene | $^1B_{3u}$ | 7.93 | 5.90 | 5.80 | 6.72 | 8.23 | 5.95 | 5.85 | 6.76 | 8.27 |
| butadiene | $^1B_u$ | 6.22 | 5.39 | | 5.38 | | 5.96 | | 5.96 | 7.33 |

**Table S2:** Continued

| | state | ref | BSE/SCF-LOSC | | | | BSE-TDA/SCF-LOSC | | | |
|---|---|---|---|---|---|---|---|---|---|---|
| | | | BLYP | PBE | B3LYP | PBE0 | BLYP | PBE | B3LYP | PBE0 |
| benzene | $^1B_{2u}$ | 5.06 | | | | | | | | |
| | $^3B_{1u}$ | 4.16 | | | | | | | | |
| naphthalene | $^1B_{3u}$ | 4.00 | | | | | | | | |
| | $^3B_{2u}$ | 3.11 | | | | | | | | |
| furan | $^1B_2$ | 6.37 | | | 5.58 | | 5.74 | | 5.96 | 7.23 |
| | $^3B_2$ | 4.20 | | | 3.00 | | 3.02 | | 3.32 | 4.66 |
| hexatriene | $^1B_u$ | 5.37 | 4.60 | | | | | | | |
| | $^3B_u$ | 2.73 | 1.60 | | | | | | | |
| water | Singlet | 7.62 | 6.85 | 7.01 | 7.42 | 9.60 | 6.90 | 7.06 | 7.46 | 9.63 |
| | Triplet | 7.25 | 5.97 | 6.13 | 6.62 | 8.82 | 6.02 | 6.18 | 6.66 | 8.85 |
| pNA | $^1A_1$ | 4.39 | | | 4.08 | 5.25 | | | 4.18 | 5.35 |
| DMABN | $^1A_1$ | 4.86 | | | | 5.48 | | | | 5.57 |

**Table S3:** Excitation energies of molecules in the Truhlar-Gagliardi test set[S1] obtained from BSE/$G_0W_0$ and BSE-TDA/$G_0W_0$ based on different starting points. The aug-cc-pVTZ basis set was used except for naphthalene, pNA and DMABN that were calculated with the aug-cc-pVDZ basis set. B-TCNE was not included because of computational cost. All values in eV.

| | state | ref | BSE/$G_0W_0$ | | | | | BSE-TDA/$G_0W_0$ | | | | |
|---|---|---|---|---|---|---|---|---|---|---|---|---|
| | | | HF | BLYP | PBE | B3LYP | PBE0 | HF | BLYP | PBE | B3LYP | PBE0 |
| acetaldehyde | $^1A''$ | 4.31 | 5.53 | 2.67 | 2.73 | 3.24 | 3.40 | 5.57 | 2.73 | 2.79 | 3.29 | 3.45 |
| acetone | $^1A_2$ | 4.47 | 5.97 | 2.74 | 2.81 | 3.25 | 3.39 | 6.00 | 2.79 | 2.86 | 3.30 | 3.44 |
| formaldehyde | $^1A_2$ | 3.98 | 5.11 | 2.46 | 2.52 | 2.91 | 3.06 | 5.15 | 2.53 | 2.58 | 2.97 | 3.12 |
| pyrazine | $^1B_{3u}$ | 4.15 | 5.36 | 2.77 | 2.81 | 3.26 | 3.39 | 5.41 | 2.87 | 2.91 | 3.35 | 3.48 |
| pyridazine | $^1B_1$ | 3.83 | 4.83 | 2.26 | 2.31 | 2.82 | 2.97 | 4.90 | 2.41 | 2.45 | 2.94 | 3.09 |
| pyridine | $^1B_1$ | 4.95 | 6.50 | 3.56 | 3.63 | 4.09 | 4.24 | 6.55 | 3.66 | 3.72 | 4.17 | 4.32 |
| pyrimidine | $^1B_1$ | 4.44 | 5.63 | 3.09 | 3.14 | 3.60 | 3.74 | 5.67 | 3.15 | 3.21 | 3.65 | 3.80 |
| s-tetrazine | $^1B_{3u}$ | 2.47 | 2.95 | 0.92 | 0.95 | 1.46 | 1.58 | 3.03 | 1.12 | 1.14 | 1.60 | 1.72 |
| ethylene | $^1B_{3u}$ | 7.93 | 7.67 | 6.16 | 6.15 | 6.46 | 6.52 | 7.67 | 6.17 | 6.16 | 6.47 | 6.53 |
| butadiene | $^1B_u$ | 6.22 | 6.72 | 5.02 | 5.05 | 5.34 | 5.42 | 6.72 | 5.31 | 5.29 | 5.61 | 5.67 |
| benzene | $^1B_{2u}$ | 5.06 | 6.93 | 5.54 | 5.53 | 5.82 | 5.87 | 6.93 | 5.54 | 5.53 | 5.82 | 5.87 |
| | $^3B_{1u}$ | 4.16 | 6.85 | 2.45 | 5.37 | 5.68 | 5.74 | 6.86 | 5.39 | 5.38 | 5.69 | 5.74 |

**Table S3:** Continued

| | state | ref | BSE/$G_0W_0$ HF | BLYP | PBE | B3LYP | PBE0 | BSE-TDA/$G_0W_0$ HF | BLYP | PBE | B3LYP | PBE0 |
|---|---|---|---|---|---|---|---|---|---|---|---|---|
| naphthalene | $^1B_{3u}$ | 4.00 | 5.05 | 3.62 | 3.64 | 3.95 | 4.03 | 5.25 | 3.67 | 3.69 | 4.00 | 4.07 |
| | $^3B_{2u}$ | 3.11 | 3.53 | 1.72 | 1.74 | 2.14 | 2.23 | 3.72 | 2.19 | 2.21 | 2.52 | 2.60 |
| furan | $^1B_2$ | 6.37 | 6.52 | 5.10 | 5.07 | 5.39 | 5.43 | 6.52 | 5.10 | 5.07 | 5.39 | 5.44 |
| | $^3B_2$ | 4.20 | 4.63 | 2.49 | 2.48 | 2.84 | 2.90 | 4.85 | 2.88 | 2.87 | 3.19 | 3.24 |
| hexatriene | $^1B_u$ | 5.37 | 5.65 | 4.09 | 4.11 | 4.44 | 4.52 | 5.91 | 4.67 | 4.69 | 4.96 | 5.03 |
| | $^3B_u$ | 2.73 | 3.41 | 0.68 | 0.69 | 1.40 | 1.52 | 3.65 | 1.56 | 1.57 | 1.98 | 2.06 |
| water | Singlet | 7.62 | 8.13 | 5.58 | 5.64 | 6.08 | 6.25 | 8.14 | 5.63 | 5.69 | 6.13 | 6.29 |
| | Triplet | 7.25 | 7.66 | 4.71 | 4.77 | 5.29 | 5.48 | 7.68 | 4.77 | 4.83 | 5.34 | 5.52 |
| pNA | $^1A_1$ | 4.39 | 4.75 | 1.98 | 2.04 | 2.80 | 3.02 | 4.92 | 2.02 | 2.08 | 2.83 | 3.05 |
| DMABN | $^1A_1$ | 4.86 | 5.14 | 3.55 | 3.57 | 3.85 | 3.92 | 5.15 | 3.56 | 3.59 | 3.86 | 3.92 |

**Table S4:** Excitation energies of molecules in the Truhlar-Gagliardi test set[S1] obtained from TDDFT and TDDFT-TDA based on different starting points. The aug-cc-pVTZ basis set was used except for naphthalene, pNA and DMABN that were calculated with the aug-cc-pVDZ basis set. B-TCNE was not included because of computational cost. All values in eV.

| | state | ref | TDDFT HF | BLYP | PBE | B3LYP | PBE0 | TDDFT-TDA HF | BLYP | PBE | B3LYP | PBE0 |
|---|---|---|---|---|---|---|---|---|---|---|---|---|
| acetaldehyde | $^1A''$ | 4.31 | 4.86 | 4.19 | 4.18 | 4.31 | 4.32 | 5.03 | 4.21 | 4.19 | 4.33 | 4.35 |
| acetone | $^1A_2$ | 4.47 | 5.12 | 4.28 | 4.28 | 4.45 | 4.48 | 5.29 | 4.30 | 4.30 | 4.48 | 4.51 |
| formaldehyde | $^1A_2$ | 3.98 | 4.44 | 3.86 | 3.84 | 3.96 | 3.97 | 4.62 | 3.88 | 3.86 | 3.99 | 4.00 |
| pyrazine | $^1B_{3u}$ | 4.15 | 4.95 | 3.58 | 3.53 | 3.94 | 3.97 | 5.13 | 3.62 | 3.57 | 3.99 | 4.03 |
| pyridazine | $^1B_1$ | 3.83 | 4.74 | 3.12 | 3.08 | 3.55 | 3.62 | 4.95 | 3.18 | 3.14 | 3.63 | 3.70 |
| pyridine | $^1B_1$ | 4.95 | 5.89 | 4.36 | 4.33 | 4.78 | 4.85 | 6.14 | 4.40 | 4.37 | 4.83 | 4.90 |
| pyrimidine | $^1B_1$ | 4.44 | 5.76 | 3.83 | 3.79 | 4.29 | 4.35 | 5.91 | 3.85 | 3.81 | 4.32 | 4.39 |
| s-tetrazine | $^1B_{3u}$ | 2.47 | 3.28 | 1.87 | 1.80 | 2.22 | 2.25 | 3.50 | 1.92 | 1.87 | 2.30 | 2.33 |
| ethylene | $^1B_{3u}$ | 7.93 | 7.16 | 6.25 | 6.49 | 6.64 | 6.89 | 7.17 | 6.25 | 6.49 | 6.64 | 6.89 |
| butadiene | $^1B_u$ | 6.22 | 5.99 | 5.33 | 5.50 | 5.72 | 5.96 | 6.21 | 5.33 | 5.57 | 5.72 | 5.97 |
| benzene | $^1B_{2u}$ | 5.06 | 5.84 | 5.23 | 5.28 | 5.41 | 5.50 | 6.04 | 5.24 | 5.29 | 5.44 | 5.53 |
| | $^3B_{1u}$ | 4.16 | -2.09 | 4.08 | 4.05 | 3.85 | 3.65 | 3.43 | 4.27 | 4.26 | 4.21 | 4.14 |
| naphthalene | $^1B_{3u}$ | 4.00 | 4.80 | 4.09 | 4.13 | 4.40 | 4.50 | 5.13 | 4.26 | 4.30 | 4.51 | 4.60 |
| | $^3B_{2u}$ | 3.11 | -2.66 | 2.93 | 2.91 | 2.83 | 2.69 | 2.70 | 3.04 | 3.04 | 3.10 | 3.07 |

**Table S4:** Continued

| | | | TDDFT | | | | | TDDFT-TDA | | | | |
|---|---|---|---|---|---|---|---|---|---|---|---|---|
| | state | ref | HF | BLYP | PBE | B3LYP | PBE0 | HF | BLYP | PBE | B3LYP | PBE0 |
| furan | $^1B_2$ | 6.37 | 6.04 | 5.12 | 5.35 | 5.55 | 5.79 | 6.05 | 5.12 | 5.35 | 5.55 | 5.79 |
| | $^3B_2$ | 4.20 | -0.32 | 4.03 | 4.03 | 3.86 | 3.74 | 3.47 | 4.17 | 4.18 | 4.12 | 4.08 |
| hexatriene | $^1B_u$ | 5.37 | 5.18 | 4.48 | 4.52 | 4.70 | 4.78 | 5.46 | 4.88 | 4.99 | 5.10 | 5.18 |
| | $^3B_u$ | 2.73 | -2.47 | 2.43 | 2.39 | 2.26 | 2.07 | 2.26 | 2.59 | 2.57 | 2.61 | 2.55 |
| water | Singlet | 7.62 | 8.67 | 6.27 | 6.41 | 6.93 | 7.19 | 8.71 | 6.28 | 6.42 | 6.95 | 7.20 |
| | Triplet | 7.25 | 7.91 | 5.97 | 6.07 | 6.57 | 6.77 | 8.04 | 5.99 | 6.09 | 6.59 | 6.80 |
| pNA | $^1A_1$ | 4.39 | 5.12 | 3.52 | 3.56 | 3.96 | 4.06 | 5.36 | 3.64 | 3.65 | 3.99 | 4.08 |
| DMABN | $^1A_1$ | 4.86 | 5.27 | 3.96 | 3.96 | 4.35 | 4.44 | 5.51 | 3.99 | 4.04 | 4.44 | 4.54 |

**Table S5:** Excitation energies of molecules in the Truhlar-Gagliardi test set[S1] obtained from BSE/ev$GW$ and BSE-TDA/ev$GW$ based on different starting points. The aug-cc-pVTZ basis set was used except for naphthalene, pNA and DMABN that were calculated with the aug-cc-pVDZ basis set. B-TCNE was not included because of computational cost. All values in eV.

| | | | BSE/ev$GW$ | | | | | BSE-TDA/ev$GW$ | | | | |
|---|---|---|---|---|---|---|---|---|---|---|---|---|
| | state | ref | HF | BLYP | PBE | B3LYP | PBE0 | HF | BLYP | PBE | B3LYP | PBE0 |
| acetaldehyde | $^1A''$ | 4.31 | 5.46 | 4.02 | 4.04 | 4.03 | 4.08 | 5.44 | 4.11 | 4.15 | 4.12 | 4.16 |
| acetone | $^1A_2$ | 4.47 | 5.90 | 4.01 | 4.06 | 3.97 | 3.98 | 5.86 | 4.15 | 4.19 | 4.08 | 4.10 |
| formaldehyde | $^1A_2$ | 3.98 | 5.04 | 3.68 | 3.73 | 3.65 | 3.69 | 5.05 | 3.75 | 3.80 | 3.72 | 3.76 |
| pyrazine | $^1B_{3u}$ | 4.15 | 5.25 | 3.86 | 3.87 | 3.91 | 3.95 | 5.25 | 3.98 | 3.98 | 4.02 | 4.05 |
| pyridazine | $^1B_1$ | 3.83 | 4.69 | 3.52 | 3.54 | 3.54 | 3.58 | 4.71 | 3.66 | 3.68 | 3.68 | 3.73 |
| pyridine | $^1B_1$ | 4.95 | 6.43 | 4.72 | 4.75 | 4.77 | 4.80 | 6.41 | 4.87 | 4.91 | 4.90 | 4.94 |
| pyrimidine | $^1B_1$ | 4.44 | 5.53 | 4.24 | 4.25 | 4.28 | 4.31 | 5.51 | 4.34 | 4.36 | 4.37 | 4.41 |
| s-tetrazine | $^1B_{3u}$ | 2.47 | 2.75 | 2.12 | 2.12 | 2.15 | 2.17 | | 2.25 | 2.25 | 2.28 | 2.30 |
| ethylene | $^1B_{3u}$ | 7.93 | 7.68 | 6.65 | 6.60 | 6.74 | 6.75 | 7.70 | 6.69 | 6.64 | 6.77 | 6.78 |
| butadiene | $^1B_u$ | 6.22 | 6.72 | 5.79 | 5.75 | 5.78 | 5.79 | 6.74 | 5.83 | 5.78 | 5.90 | 5.91 |
| benzene | $^1B_{2u}$ | 5.06 | 6.20 | 5.04 | 5.06 | 5.06 | 5.11 | 6.93 | 6.11 | 6.05 | 6.14 | 6.12 |
| | $^3B_{1u}$ | 4.16 | 4.76 | 3.24 | 3.26 | 3.31 | 3.37 | 6.86 | 5.96 | 5.90 | 6.00 | 6.00 |
| naphthalene | $^1B_{3u}$ | 4.00 | 4.82 | 4.30 | 4.30 | 4.31 | 4.31 | 5.14 | 4.38 | 4.37 | 4.40 | 4.40 |
| | $^3B_{2u}$ | 3.11 | 3.24 | 2.45 | 2.45 | 2.50 | 2.50 | 3.62 | 2.87 | 2.87 | 2.91 | 2.92 |
| furan | $^1B_2$ | 6.37 | 6.52 | 5.55 | 5.49 | 5.62 | 5.62 | 6.53 | 5.60 | 5.54 | 5.67 | 5.67 |
| | $^3B_2$ | 4.20 | 4.63 | 3.20 | 3.18 | 3.22 | 3.21 | 4.80 | 3.58 | 3.56 | 3.60 | 3.58 |

**Table S5:** Continued

| | state | ref | BSE/ev$GW$ | | | | | BSE-TDA/ev$GW$ | | | | |
|---|---|---|---|---|---|---|---|---|---|---|---|---|
| | | | HF | BLYP | PBE | B3LYP | PBE0 | HF | BLYP | PBE | B3LYP | PBE0 |
| hexatriene | $^1B_u$ | 5.37 | 5.63 | 4.88 | 4.88 | 4.89 | 4.91 | 5.87 | 5.38 | 5.35 | 5.41 | 5.41 |
| | $^3B_u$ | 2.73 | 3.40 | 1.79 | 1.77 | 1.93 | 1.96 | 3.62 | 2.32 | 2.31 | 2.42 | 2.43 |
| water | Singlet | 7.62 | 8.03 | 6.73 | 6.75 | 6.77 | 6.84 | 8.03 | 6.80 | 6.82 | 6.83 | 6.90 |
| | Triplet | 7.25 | 7.57 | 5.87 | 5.88 | 5.98 | 6.07 | 7.57 | 5.94 | 5.96 | 6.04 | 6.14 |
| pNA | $^1A_1$ | 4.39 | 4.49 | 3.77 | 3.82 | 3.78 | 3.85 | 4.52 | 3.85 | 3.90 | 3.84 | 3.91 |
| DMABN | $^1A_1$ | 4.86 | 4.87 | 4.33 | 4.32 | 4.33 | 4.33 | 5.08 | 4.19 | 4.17 | 4.18 | 4.18 |

**Table S6:** Mean absolute errors (MAEs) and mean signed errors (MSEs) of excitation energies in Truhlar-Gagliardi test set obtained from BSE/LOSC, BSE/$G_0W_0$, TDDFT, BSE/ev$GW$, BSE-TDA/LOSC, BSE-TDA/$G_0W_0$, TDDFT-TDA and BSE-TDA/ev$GW$ based on HF, BLYP, PBE, B3LYP and PBE0. All values in eV. Geometries were taken from Ref. S1. Reference values for pNA and DMABN were taken from Ref. S2 and for remaining molecules were taken from Ref. S3. The aug-cc-pVDZ basis set was used for naphthalene, pNA and DMABN, and the aug-cc-pVTZ basis set was used for the remaining systems. B-TCNE was excluded considering the computational cost. Total MAEs and total MSEs were calculated by averaging all systems.

| | | valence | | Rydberg | | CT | |
|---|---|---|---|---|---|---|---|
| | | MAE | MSE | MAE | MSE | MAE | MSE |
| BLYP | BSE/LOSC | 1.09 | -1.06 | 0.92 | -0.92 | 0.77 | -0.77 |
| | BSE-TDA/LOSC | 0.89 | -0.81 | 0.87 | -0.87 | 0.65 | -0.65 |
| PBE | BSE/LOSC | 1.13 | -1.09 | 0.75 | -0.75 | 0.75 | -0.75 |
| | BSE-TDA/LOSC | 0.94 | -0.83 | 0.71 | -0.71 | 0.64 | -0.64 |
| B3LYP | BSE/LOSC | 0.67 | -0.60 | 0.35 | -0.35 | 0.40 | -0.40 |
| | BSE-TDA/LOSC | 0.53 | -0.39 | 0.30 | -0.30 | 0.31 | -0.31 |
| PBE0 | BSE/LOSC | 0.60 | -0.51 | 0.20 | -0.08 | 0.31 | -0.31 |
| | BSE-TDA/LOSC | 0.46 | -0.30 | 0.20 | -0.04 | 0.21 | -0.21 |
| HF | BSE/$G_0W_0$ | 1.08 | 0.98 | 0.46 | 0.46 | 0.32 | 0.32 |
| | BSE-TDA/$G_0W_0$ | 1.11 | 1.04 | 0.48 | 0.48 | 0.41 | 0.41 |
| BLYP | BSE/$G_0W_0$ | 1.37 | -1.34 | 2.29 | -2.29 | 1.86 | -1.86 |
| | BSE-TDA/$G_0W_0$ | 1.22 | -1.00 | 2.23 | -2.23 | 1.83 | -1.83 |
| PBE | BSE/$G_0W_0$ | 1.32 | -1.17 | 2.23 | -2.23 | 1.82 | -1.82 |
| | BSE-TDA/$G_0W_0$ | 1.20 | -0.98 | 2.18 | -2.18 | 1.79 | -1.79 |
| B3LYP | BSE/$G_0W_0$ | 1.00 | -0.76 | 1.75 | -1.75 | 1.30 | -1.30 |
| | BSE-TDA/$G_0W_0$ | 0.89 | -0.60 | 1.70 | -1.70 | 1.28 | -1.28 |

**Table S6:** Continued

| | | valence | | Rydberg | | CT | |
|---|---|---|---|---|---|---|---|
| | | MAE | MSE | MAE | MSE | MAE | MSE |
| PBE0 | BSE/$G_0W_0$ | 0.91 | -0.65 | 1.57 | -1.57 | 1.16 | -1.16 |
| | BSE-TDA/$G_0W_0$ | 0.81 | -0.50 | 1.53 | -1.53 | 1.14 | -1.14 |
| HF | TDDFT | 1.62 | -0.85 | 0.85 | 0.85 | 0.57 | 0.57 |
| | TDDFT-TDA | 0.81 | 0.37 | 0.94 | 0.94 | 0.81 | 0.81 |
| BLYP | TDDFT | 0.50 | -0.48 | 1.31 | -1.31 | 0.89 | -0.89 |
| | TDDFT-TDA | 0.48 | -0.40 | 1.30 | -1.30 | 0.81 | -0.81 |
| PBE | TDDFT | 0.49 | -0.46 | 1.19 | -1.19 | 0.86 | -0.86 |
| | TDDFT-TDA | 0.46 | -0.37 | 1.18 | -1.18 | 0.78 | -0.78 |
| B3LYP | TDDFT | 0.34 | -0.28 | 0.68 | -0.68 | 0.47 | -0.47 |
| | TDDFT-TDA | 0.28 | -0.16 | 0.67 | -0.67 | 0.41 | -0.41 |
| PBE0 | TDDFT | 0.31 | -0.24 | 0.46 | -0.46 | 0.37 | -0.37 |
| | TDDFT-TDA | 0.23 | -0.10 | 0.43 | -0.43 | 0.32 | -0.32 |
| HF | BSE/ev$GW$ | 0.78 | 0.72 | 0.37 | 0.37 | 0.06 | 0.06 |
| | BSE-TDA/ev$GW$ | 1.05 | 0.99 | 0.37 | 0.37 | 0.18 | 0.18 |
| BLYP | BSE/ev$GW$ | 0.49 | -0.48 | 1.13 | -1.13 | 0.57 | -0.57 |
| | BSE-TDA/ev$GW$ | 0.50 | -0.11 | 1.06 | -1.06 | 0.61 | -0.61 |
| PBE | BSE/ev$GW$ | 0.49 | -0.48 | 1.12 | -1.12 | 0.55 | -0.55 |
| | BSE-TDA/ev$GW$ | 0.49 | -0.11 | 1.05 | -1.05 | 0.59 | -0.59 |
| B3LYP | BSE/ev$GW$ | 0.46 | -0.45 | 1.06 | -1.06 | 0.57 | -0.57 |
| | BSE-TDA/ev$GW$ | 0.48 | -0.08 | 1.00 | -1.00 | 0.61 | -0.61 |
| PBE0 | BSE/ev$GW$ | 0.45 | -0.43 | 0.98 | -0.98 | 0.54 | -0.54 |
| | BSE-TDA/ev$GW$ | 0.46 | -0.06 | 0.92 | -0.92 | 0.58 | -0.58 |

# 3 Results of Stein CT Test Set

**Table S7:** Excitation energies of charge transfer systems in the Stein CT test set[S4] obtained from BSE/post-LOSC and BSE-TDA/post-LOSC based on different starting points. Gas phase results were taken as the reference. The cc-pVDZ basis set was used. All values in eV.

| | | BSE/post-LOSC | | | | BSE-TDA/post-LOSC | | | |
|---|---|---|---|---|---|---|---|---|---|
| | ref | BLYP | PBE | B3LYP | PBE0 | BLYP | PBE | B3LYP | PBE0 |
| anthracene | 2.05 | 2.18 | 2.19 | 2.04 | 2.05 | 2.36 | 2.36 | 2.17 | 2.17 |
| 9-cyano | 2.33 | 2.09 | 2.14 | 1.86 | 1.89 | 2.17 | 2.21 | 1.90 | 1.91 |
| 9-cholo | 2.06 | 2.08 | 2.08 | 1.94 | 1.91 | 2.22 | 2.22 | 2.04 | 1.99 |
| 9-carbo-methoxy | 2.16 | 2.29 | 2.18 | 1.98 | 1.98 | 2.41 | 2.29 | 2.06 | 2.04 |
| 9-methyl | 1.87 | 2.05 | 2.02 | 1.94 | 1.87 | 2.24 | 2.20 | 2.08 | 2.00 |
| 9,10-dimethyl | 1.76 | 2.14 | 2.09 | 2.06 | 2.05 | 2.39 | 2.32 | 2.27 | 2.24 |
| 9-formyl | 2.22 | 2.19 | 2.31 | 2.12 | 2.16 | 2.28 | 2.39 | 2.19 | 2.22 |
| 9-formyl, 10-chloro | 2.28 | 2.13 | 2.01 | 2.14 | 2.19 | 2.21 | 2.09 | 2.19 | 2.24 |
| benzene | 3.91 | 2.48 | 2.51 | 2.82 | 2.94 | 2.48 | 2.51 | 2.82 | 2.94 |
| toluene | 3.68 | 2.46 | 2.43 | 2.60 | 2.67 | 2.46 | 2.44 | 2.62 | 2.69 |
| o-xylene | 3.47 | 2.29 | 2.27 | 2.43 | 2.43 | 2.29 | 2.28 | 2.44 | 2.44 |
| naphthalene | 2.92 | 1.98 | 1.91 | 2.10 | 2.15 | 1.99 | 1.91 | 2.11 | 2.16 |

**Table S8:** Excitation energies of charge transfer systems in the Stein CT test set[S4] obtained from BSE/SCF-LOSC and BSE-TDA/SCF-LOSC based on different starting points. Gas phase results were taken as the reference. The cc-pVDZ basis set was used. All values in eV. Some results are missing because of the convergence issue in SCF-LOSC.

| | | BSE/SCF-LOSC | | | | BSE-TDA/SCF-LOSC | | | |
|---|---|---|---|---|---|---|---|---|---|
| | ref | BLYP | PBE | B3LYP | PBE0 | BLYP | PBE | B3LYP | PBE0 |
| anthracene | 2.05 | | | | 2.82 | | | | 2.89 |
| 9-cyano | 2.33 | | | | 2.80 | | | | 2.81 |
| 9-cholo | 2.06 | | | | 2.74 | | | | 2.77 |
| 9-carbo-methoxy | 2.16 | | | 1.77 | 2.81 | | | 1.81 | 2.84 |
| 9-methyl | 1.87 | 1.66 | 1.65 | | 2.70 | 1.73 | 1.72 | | 2.76 |
| 9,10-dimethyl | 1.76 | | | | | | | | |
| 9-formyl | 2.22 | | 1.82 | 1.98 | 3.05 | | 1.84 | 2.01 | 3.07 |
| 9-formyl, 10-chloro | 2.28 | | 1.92 | 2.11 | 3.09 | | 1.93 | 2.13 | 3.11 |
| benzene | 3.91 | | | | 4.02 | | | | 4.02 |
| toluene | 3.68 | 2.45 | 2.44 | 2.57 | 3.70 | 2.45 | 2.44 | 2.58 | 3.71 |
| o-xylene | 3.47 | 2.16 | | 2.41 | 3.49 | 2.16 | | 2.42 | 3.49 |
| naphthalene | 2.92 | | | 2.07 | 3.24 | | | 2.07 | 3.24 |

**Table S8:** Continued

| | | BSE/SCF-LOSC | | | | BSE-TDA/SCF-LOSC | | | |
|---|---|---|---|---|---|---|---|---|---|
| | ref | BLYP | PBE | B3LYP | PBE0 | BLYP | PBE | B3LYP | PBE0 |

**Table S9:** Excitation energies of charge transfer systems in the Stein CT test set[S4] obtained from BSE/$G_0W_0$ and BSE-TDA/$G_0W_0$ based on different starting points. Gas phase results were taken as the reference. The cc-pVDZ basis set was used. All values in eV.

| | | BSE/$G_0W_0$ | | | | | BSE-TDA/$G_0W_0$ | | | | |
|---|---|---|---|---|---|---|---|---|---|---|---|
| | ref | HF | BLYP | PBE | B3LYP | PBE0 | HF | BLYP | PBE | B3LYP | PBE0 |
| anthracene | 2.05 | 2.02 | 0.95 | 0.90 | 1.41 | 1.47 | 2.06 | 1.21 | 1.16 | 1.57 | 1.61 |
| 9-cyano | 2.33 | 2.39 | 1.33 | 1.34 | 1.34 | 1.58 | 2.40 | 1.45 | 1.51 | 1.37 | 1.60 |
| 9-cholo | 2.06 | 2.09 | 0.69 | 0.65 | 1.30 | 1.40 | 2.11 | 0.94 | 0.89 | 1.42 | 1.49 |
| 9-carbo-methoxy | 2.16 | 2.17 | 0.61 | 0.55 | 1.30 | 1.41 | 2.18 | 0.82 | 0.76 | 1.39 | 1.49 |
| 9-methyl | 1.87 | 1.86 | 0.72 | 0.67 | 1.22 | 1.29 | 1.89 | 1.03 | 0.99 | 1.40 | 1.44 |
| 9,10-dimethyl | 1.76 | 1.83 | 1.01 | 0.97 | 1.39 | 1.43 | 1.90 | 1.36 | 1.32 | 1.63 | 1.65 |
| 9-formyl | 2.22 | 2.24 | 0.72 | 0.69 | 1.43 | 1.55 | 2.26 | 0.87 | 0.79 | 1.50 | 1.60 |
| 9-formyl, 10-chloro | 2.28 | 2.33 | 0.68 | 0.66 | 1.47 | 1.61 | 2.34 | 0.81 | 0.77 | 1.53 | 1.66 |
| benzene | 3.91 | 3.74 | 2.72 | 2.69 | 3.22 | 3.26 | 3.74 | 2.73 | 2.70 | 3.23 | 3.27 |
| toluene | 3.68 | 3.43 | 2.18 | 2.15 | 2.86 | 2.91 | 3.43 | 2.21 | 2.18 | 2.87 | 2.93 |
| o-xylene | 3.47 | 3.15 | 1.82 | 1.78 | 2.52 | 2.59 | 3.15 | 1.83 | 1.79 | 2.53 | 2.59 |
| naphthalene | 2.92 | 2.74 | 1.90 | 1.91 | 2.33 | 2.35 | 2.75 | 1.90 | 1.92 | 2.33 | 2.36 |

**Table S10:** Excitation energies of charge transfer systems in the Stein CT test set[S4] obtained from TDDFT and TDDFT-TDA based on different starting points. Gas phase results were taken as the reference. The cc-pVDZ basis set was used. All values in eV.

| | | TDDFT | | | | | TDDFT-TDA | | | | |
|---|---|---|---|---|---|---|---|---|---|---|---|
| | ref | HF | BLYP | PBE | B3LYP | PBE0 | HF | BLYP | PBE | B3LYP | PBE0 |
| anthracene | 2.05 | 2.83 | 1.46 | 1.46 | 1.55 | 1.59 | 2.88 | 1.75 | 1.74 | 1.73 | 1.74 |
| 9-cyano | 2.33 | 3.19 | 0.72 | 0.72 | 0.82 | 0.91 | 3.23 | 0.91 | 0.90 | 0.87 | 0.94 |
| 9-cholo | 2.06 | 2.92 | 1.23 | 1.23 | 1.32 | 1.36 | 2.95 | 1.49 | 1.48 | 1.46 | 1.48 |
| 9-carbo-methoxy | 2.16 | 3.00 | 1.13 | 1.12 | 1.23 | 1.28 | 3.02 | 1.35 | 1.34 | 1.34 | 1.37 |
| 9-methyl | 1.87 | 2.65 | 1.34 | 1.34 | 1.41 | 1.44 | 2.70 | 1.64 | 1.64 | 1.61 | 1.61 |
| 9,10-dimethyl | 1.76 | 2.59 | 1.60 | 1.60 | 1.67 | 1.70 | 2.67 | 1.96 | 1.96 | 1.93 | 1.93 |

**Table S10:** Continued

| | ref | TDDFT | | | | | TDDFT-TDA | | | | |
|---|---|---|---|---|---|---|---|---|---|---|---|
| | | HF | BLYP | PBE | B3LYP | PBE0 | HF | BLYP | PBE | B3LYP | PBE0 |
| 9-formyl | 2.22 | 3.07 | 0.87 | 0.79 | 1.27 | 1.33 | 3.09 | 0.87 | 0.79 | 1.36 | 1.40 |
| 9-formyl, 10-chloro | 2.28 | 3.17 | 0.85 | 0.78 | 1.22 | 1.30 | 3.19 | 0.85 | 0.78 | 1.30 | 1.35 |
| benzene | 3.91 | 4.64 | 1.42 | 1.42 | 1.98 | 2.14 | 4.65 | 1.42 | 1.43 | 1.98 | 2.14 |
| toluene | 3.68 | 4.32 | 1.38 | 1.37 | 1.82 | 1.95 | 4.34 | 1.42 | 1.41 | 1.84 | 1.97 |
| o-xylene | 3.47 | 4.08 | 1.07 | 1.06 | 1.54 | 1.68 | 4.09 | 1.08 | 1.07 | 1.55 | 1.68 |
| naphthalene | 2.92 | 3.56 | 0.34 | 0.36 | 0.90 | 1.07 | 3.57 | 0.34 | 0.36 | 0.91 | 1.08 |

# 4 Results of Rydberg Excitations

**Table S11:** Rydberg excitation energies of Be, $B^+$ and Mg obtained from BSE/post-LOSC and BSE-TDA/post-LOSC based on different starting points. Reference values were from Ref. S5. The aug-cc-pVQZ basis set was used. All values in eV.

| | state | ref | BSE/post-LOSC | | | | BSE-TDA/post-LOSC | | | |
|---|---|---|---|---|---|---|---|---|---|---|
| | | | BLYP | PBE | B3LYP | PBE0 | BLYP | PBE | B3LYP | PBE0 |
| Be | triplet 2s→3s | 6.46 | 5.44 | 5.59 | 5.52 | 5.72 | 5.47 | 5.62 | 5.55 | 5.75 |
| | singlet 2s→3s | 6.78 | 6.25 | 6.50 | 6.45 | 6.62 | 6.30 | 6.54 | 6.49 | 6.65 |
| $B^+$ | triplet 2s→3s | 16.09 | 14.26 | 14.56 | 14.56 | 14.84 | 14.30 | 14.60 | 14.59 | 14.87 |
| | singlet 2s→3s | 17.06 | 15.90 | 16.19 | 16.06 | 16.27 | 15.94 | 16.23 | 16.10 | 16.31 |
| Mg | triplet 3s→4s | 5.11 | 4.41 | 4.60 | 4.56 | 4.73 | 4.44 | 4.63 | 4.58 | 4.75 |
| | singlet 3s→4s | 5.39 | 5.33 | 5.34 | 5.31 | 5.44 | 5.38 | 5.38 | 5.35 | 5.47 |

**Table S12:** Rydberg excitation energies of Be, $B^+$ and Mg obtained from BSE/$G_0W_0$ and BSE-TDA/$G_0W_0$ based on different starting points. Reference values were from Ref. S5. The aug-cc-pVQZ basis set was used. All values in eV.

| | state | ref | BSE/$G_0W_0$ | | | | | BSE-TDA/$G_0W_0$ | | | | |
|---|---|---|---|---|---|---|---|---|---|---|---|---|
| | | | HF | BLYP | PBE | B3LYP | PBE0 | HF | BLYP | PBE | B3LYP | PBE0 |
| Be | triplet 2s→3s | 6.46 | 6.24 | | | 5.50 | 5.62 | 6.26 | 5.25 | 5.28 | 5.54 | 5.65 |
| | singlet 2s→3s | 6.78 | 6.83 | 6.27 | 6.30 | 6.47 | 6.52 | 6.85 | 6.32 | 6.35 | 6.51 | 6.56 |
| $B^+$ | triplet 2s→3s | 16.09 | 15.83 | 14.29 | 14.30 | 14.82 | 14.96 | 15.85 | 14.32 | 14.33 | 14.85 | 14.99 |
| | singlet 2s→3s | 17.06 | 16.82 | 15.83 | 15.85 | 16.31 | 16.36 | 16.84 | 15.88 | 15.9 | 16.34 | 16.4 |

**Table S12:** Continued

| | state | ref | BSE/$G_0W_0$ | | | | | BSE-TDA/$G_0W_0$ | | | | |
|---|---|---|---|---|---|---|---|---|---|---|---|---|
| | | | HF | BLYP | PBE | B3LYP | PBE0 | HF | BLYP | PBE | B3LYP | PBE0 |
| Mg | triplet 3s→4s | 5.11 | 5.01 | 4.09 | 4.12 | 4.32 | 4.42 | 5.03 | 4.12 | 4.15 | 4.34 | 4.45 |
| | singlet 3s→4s | 5.39 | 5.49 | 4.96 | 5.00 | 5.11 | 5.17 | 5.5 | 5 | 5.04 | 5.14 | 5.2 |

**Table S13:** Rydberg excitation energies of Be, $B^+$ and Mg obtained from TDDFT and TDDFT-TDA based on different starting points. Reference values were from Ref. S5. The aug-cc-pVQZ basis set was used. All values in eV.

| | state | ref | TDDFT | | | | | TDDFT-TDA | | | | |
|---|---|---|---|---|---|---|---|---|---|---|---|---|
| | | | HF | BLYP | PBE | B3LYP | PBE0 | HF | BLYP | PBE | B3LYP | PBE0 |
| Be | triplet 2s→3s | 6.46 | 5.49 | 5.37 | 5.47 | 5.65 | 5.70 | 5.53 | 5.38 | 5.48 | 5.66 | 5.71 |
| | singlet 2s→3s | 6.78 | 6.13 | 5.55 | 5.75 | 5.88 | 6.03 | 6.14 | 5.56 | 5.76 | 5.89 | 6.04 |
| $B^+$ | triplet 2s→3s | 16.09 | 14.76 | 14.68 | 14.78 | 14.96 | 15.02 | 14.8 | 14.69 | 14.79 | 14.96 | 15.03 |
| | singlet 2s→3s | 17.06 | 15.82 | 15.26 | 15.45 | 15.58 | 15.74 | 15.84 | 15.29 | 15.46 | 15.6 | 15.75 |
| Mg | triplet 3s→4s | 5.11 | 4.32 | 4.45 | 4.52 | 4.67 | 4.68 | 4.35 | 4.45 | 4.53 | 4.67 | 4.68 |
| | singlet 3s→4s | 5.39 | 4.84 | 4.57 | 4.73 | 4.83 | 4.93 | 4.85 | 4.58 | 4.74 | 4.84 | 4.94 |

**Table S14:** Rydberg excitation energies of Be, $B^+$ and Mg obtained from BSE/ev$GW$ and BSE-TDA/ev$GW$ based on different starting points. Reference values were from Ref. S5. The aug-cc-pVQZ basis set was used. All values in eV.

| | state | ref | BSE/ev$GW$ | | | | | BSE-TDA/ev$GW$ | | | | |
|---|---|---|---|---|---|---|---|---|---|---|---|---|
| | | | HF | BLYP | PBE | B3LYP | PBE0 | HF | BLYP | PBE | B3LYP | PBE0 |
| Be | triplet 2s→3s | 6.46 | 6.29 | 5.60 | 5.59 | 5.70 | 5.77 | 6.31 | 5.63 | 5.62 | 5.74 | 5.80 |
| | singlet 2s→3s | 6.78 | 6.87 | 6.64 | 6.62 | 6.65 | 6.66 | 6.89 | 6.68 | 6.67 | 6.68 | 6.69 |
| $B^+$ | triplet 2s→3s | 16.09 | 15.87 | 14.78 | 14.81 | 14.92 | 15.01 | 15.89 | 14.82 | 14.84 | 14.95 | 15.04 |
| | singlet 2s→3s | 17.06 | 16.86 | 16.38 | 16.38 | 16.40 | 16.41 | 16.88 | 16.42 | 16.42 | 16.44 | 16.45 |
| Mg | triplet 3s→4s | 5.11 | 5.06 | 4.38 | 4.37 | 4.46 | 4.54 | 5.07 | 4.41 | 4.40 | 4.49 | 4.56 |
| | singlet 3s→4s | 5.39 | 5.53 | 5.23 | 5.24 | 5.24 | 5.27 | 5.55 | 5.27 | 5.28 | 5.27 | 5.30 |

# 5 Fundamental gaps obtained from $G_0W_0$, post-SCF LOSC and ev$GW$

**Table S15:** Fundamental gaps of molecules in the Truhlar-Gagliardi test set[S1] obtained from $G_0W_0$, post-SCF LOSC and ev$GW$ based on BLYP. The aug-cc-pVTZ basis set was used except for naphthalene, pNA and DMABN that were calculated with the aug-cc-pVDZ basis set. B-TCNE was not included because of computational cost. All values in eV.

| | $G_0W_0$@BLYP | post-LOSC@BLYP | ev$GW$@BLYP |
|---|---|---|---|
| acetaldehyde | 10.80 | 11.72 | 12.25 |
| acetone | 10.40 | 11.65 | 11.78 |
| formaldehyde | 11.30 | 11.53 | 12.63 |
| pyrazine | 8.98 | 10.25 | 10.12 |
| pyridazine | 8.46 | 8.63 | 9.73 |
| pyridine | 9.59 | 10.68 | 10.79 |
| pyrimidine | 9.33 | 10.39 | 10.53 |
| s-tetrazine | 7.61 | 7.58 | 8.81 |
| ethylene | 12.16 | 12.27 | 12.92 |
| butadiene | 9.47 | 9.84 | 10.20 |
| benzene | 10.14 | 9.63 | 10.86 |
| naphthalene | 7.88 | 8.13 | 8.58 |
| furan | 10.42 | 10.48 | 11.12 |
| hexatriene | 7.89 | 8.50 | 8.62 |
| water | 12.81 | 14.19 | 13.99 |
| pNA | 7.27 | 7.93 | 8.30 |
| DMABN | 7.90 | 8.60 | 8.74 |

**Table S16:** Fundamental gaps of molecules in the Truhlar-Gagliardi test set[S1] obtained from $G_0W_0$, post-SCF LOSC and ev$GW$ based on PBE. The aug-cc-pVTZ basis set was used except for naphthalene, pNA and DMABN that were calculated with the aug-cc-pVDZ basis set. B-TCNE was not included because of computational cost. All values in eV.

| | $G_0W_0$@PBE | post-LOSC@PBE | ev$GW$@PBE |
|---|---|---|---|
| acetaldehyde | 10.89 | 11.64 | 12.29 |
| acetone | 10.48 | 11.58 | 11.83 |
| formaldehyde | 11.43 | 11.46 | 12.72 |
| pyrazine | 9.05 | 10.13 | 10.15 |
| pyridazine | 8.54 | 8.56 | 9.78 |
| pyridine | 9.68 | 10.57 | 10.84 |
| pyrimidine | 9.41 | 10.28 | 10.56 |
| s-tetrazine | 7.66 | 7.43 | 8.83 |

**Table S16:** Continued

| | $G_0W_0$@PBE | post-LOSC@PBE | ev$GW$@PBE |
|---|---|---|---|
| ethylene | 12.25 | 12.37 | 12.98 |
| butadiene | 9.53 | 9.82 | 10.22 |
| benzene | 10.18 | 9.71 | 10.91 |
| naphthalene | 7.92 | 8.28 | 8.60 |
| furan | 10.46 | 10.53 | 11.13 |
| hexatriene | 7.93 | 8.51 | 8.63 |
| water | 12.89 | 14.39 | 14.03 |
| pNA | 7.27 | 8.07 | 8.27 |
| DMABN | 7.95 | 8.52 | 8.77 |

**Table S17:** Fundamental gaps of molecules in the Truhlar-Gagliardi test set[S1] obtained from $G_0W_0$, post-SCF LOSC and ev$GW$ based on B3LYP. The aug-cc-pVTZ basis set was used except for naphthalene, pNA and DMABN that were calculated with the aug-cc-pVDZ basis set. B-TCNE was not included because of computational cost. All values in eV.

| | $G_0W_0$@B3LYP | post-LOSC@B3LYP | ev$GW$@B3LYP |
|---|---|---|---|
| acetaldehyde | 11.42 | 12.22 | 12.30 |
| acetone | 10.97 | 12.06 | 11.82 |
| formaldehyde | 11.76 | 12.04 | 12.56 |
| pyrazine | 9.51 | 10.78 | 10.21 |
| pyridazine | 9.04 | 9.45 | 9.81 |
| pyridine | 10.14 | 11.25 | 10.90 |
| pyrimidine | 9.86 | 10.94 | 10.61 |
| s-tetrazine | 8.17 | 8.38 | 8.87 |
| ethylene | 12.39 | 12.55 | 12.86 |
| butadiene | 9.83 | 9.88 | 10.29 |
| benzene | 10.45 | 10.21 | 10.91 |
| naphthalene | 8.21 | 8.43 | 8.61 |
| furan | 9.55 | 9.97 | 9.83 |
| hexatriene | 8.31 | 8.67 | 8.76 |
| water | 13.04 | 14.43 | 13.75 |
| pNA | 7.78 | 8.27 | 8.37 |
| DMABN | 8.27 | 8.47 | 8.76 |

**Table S18:** Fundamental gaps of molecules in the Truhlar-Gagliardi test set[S1] obtained from $G_0W_0$, post-SCF LOSC and ev$GW$ based on PBE0. The aug-cc-pVTZ basis set was used except for naphthalene, pNA and DMABN that were calculated with the aug-cc-pVDZ basis set. B-TCNE was not included because of computational cost. All values in eV.

| | $G_0W_0$@PBE0 | post-LOSC@PBE0 | ev$GW$@PBE0 |
|---|---|---|---|
| acetaldehyde | 11.61 | 12.30 | 12.32 |
| acetone | 11.13 | 12.14 | 11.78 |
| formaldehyde | 11.94 | 12.16 | 12.61 |
| pyrazine | 9.67 | 10.81 | 10.25 |
| pyridazine | 9.23 | 9.61 | 9.85 |
| pyridine | 10.33 | 11.32 | 10.91 |
| pyrimidine | 10.04 | 10.99 | 10.63 |
| s-tetrazine | 8.32 | 8.46 | 8.92 |
| ethylene | 12.49 | 12.73 | 12.85 |
| butadiene | 9.94 | 9.98 | 10.29 |
| benzene | 10.55 | 10.39 | 10.93 |
| naphthalene | 8.30 | 8.56 | 8.63 |
| furan | 8.81 | 8.76 | 9.72 |
| hexatriene | 8.43 | 8.72 | 8.80 |
| water | 13.08 | 14.57 | 13.68 |
| pNA | 7.89 | 8.36 | 8.37 |
| DMABN | 8.39 | 8.71 | 8.79 |

# 6 Dipole moments of molecules from KS-DFT, SCF LOSC, qs$GW$ and sc$GW$

**Table S19:** Dipole moments of molecules obtained from KS-DFT, SCF LOSC, qs$GW$ and sc$GW$ based on BLYP, PBE, B3LYP and PBE0. The def2-TZVPP basis set was used. References and results of qs$GW$ and sc$GW$ were taken from Ref. S6. All values in Debye.

| | | KS-DFT | | | | SCF LOSC | | | | qs$GW$ | sc$GW$ |
|---|---|---|---|---|---|---|---|---|---|---|---|
| | ref | BLYP | PBE | B3LYP | PBE0 | BLYP | PBE | B3LYP | PBE0 | | |
| LiH | 6.02 | 5.56 | 5.60 | 5.71 | 5.76 | 5.92 | 5.90 | 5.84 | 5.89 | 5.83 | 5.90 |
| HF | 1.95 | 1.80 | 1.80 | 1.85 | 1.85 | 1.80 | 1.80 | 1.85 | 1.85 | 1.84 | 1.85 |
| LiF | 6.49 | 5.95 | 5.97 | 6.11 | 6.16 | 5.98 | 6.00 | 6.13 | 6.18 | 6.29 | 6.48 |
| CO | 0.30 | 0.17 | 0.21 | 0.07 | 0.08 | 0.17 | 0.21 | 0.07 | 0.08 | 0.07 | 0.07 |

# References

(S1) Hoyer, C. E.; Ghosh, S.; Truhlar, D. G.; Gagliardi, L. Multiconfiguration Pair-Density Functional Theory Is as Accurate as CASPT2 for Electronic Excitation. *J. Phys. Chem. Lett.* **2016**, *7*, 586–591.

(S2) Gui, X.; Holzer, C.; Klopper, W. Accuracy Assessment of GW Starting Points for Calculating Molecular Excitation Energies Using the Bethe–Salpeter Formalism. *J. Chem. Theory Comput.* **2018**, *14*, 2127–2136.

(S3) Véril, M.; Scemama, A.; Caffarel, M.; Lipparini, F.; Boggio-Pasqua, M.; Jacquemin, D.; Loos, P.-F. QUESTDB: A Database of Highly Accurate Excitation Energies for the Electronic Structure Community. *WIREs Comput. Mol. Sci.* **2021**, *11*, e1517.

(S4) Stein, T.; Kronik, L.; Baer, R. Reliable Prediction of Charge Transfer Excitations in Molecular Complexes Using Time-Dependent Density Functional Theory. *J. Am. Chem. Soc.* **2009**, *131*, 2818–2820.

(S5) Xu, X.; Yang, K. R.; Truhlar, D. G. Testing Noncollinear Spin-Flip, Collinear Spin-Flip, and Conventional Time-Dependent Density Functional Theory for Predicting Electronic Excitation Energies of Closed-Shell Atoms. *J. Chem. Theory Comput.* **2014**, *10*, 2070–2084.

(S6) Kaplan, F.; Harding, M. E.; Seiler, C.; Weigend, F.; Evers, F.; van Setten, M. J. Quasi-Particle Self-Consistent GW for Molecules. *J. Chem. Theory Comput.* **2016**, *12*, 2528–2541.
